# Supplementary material for: End-to-End Entity Resolution and Question Answering Using Differentiable Knowledge Graphs
Source: arXiv:2109.05817 source file (2021-09-13)
Supplement: Supplementary file 1 [file rigeler-appendix.pdf]

## A Model Hyperparameters

We train Rigel models using the below hyperparameters on a single GPU machine with 16GB GPU memory (AWS p3.2xlarge). WebQSP requires more than 1 hop for question answering leading to a larger knowledge graph, so we use a smaller batch size to avoid out of memory issues. Training with early stopping completes in approximately 4-7 hours depending on the model configuration used (Rigel-baseline, Rigel-ER, Rigel-E2E).

| Hyperparameter        | SIQ   | WQSP  |
|-----------------------|-------|-------|
| Batch Size            | 32    | 6     |
| Gradient Accumulation | 8     | 32    |
| Max Training Steps    | 20000 | 30000 |
| Learning Rate         | 1e-4  | 1e-4  |
| Max Number of Hops    | 1     | 3     |

Table 1: Hyperparameters for training on WebQuestionsSP (WQSP) and SimpleQuestions (SIQ)

## B Examples

The table below shows outputs of Rigel-E2E model on two questions from SimpleQuestions. In the first example, the model assigns high likelihood to the correct span and candidate entity. The inference module also assigns a high likelihood to the right relation (`instance of`), following which leads us to the correct answer entity.

In the second question, the model assigns high likelihood to `sam edwards` span, but it's not very confident and other spans such as `sam` and `edwards` receive similar scores. In addition, there's a large overlap between candidate entities of these spans; i.e. all produce candidates which are human and have `place of birth` property. This ambiguity in context leads to ground truth question entity receiving a low likelihood. Even though the right relation is predicted by the inference module, the final answer entity will be different from answer label.

---

**Question:** what is the category of the celestial object 1241 dysona?

**Question Entity:** Q137259 (1241 Dysona)

**Answer Entity** Q3863 (asteroid)

Span Likelihoods:

(**'1241 dysona', 0.965**), ('celestial', 0.013), ('celestial object', 0.011),  
( 'object', 0.009), ('1241', 0.002), ('the category', 0.0), ('what is', 0.0), ('category', 0.0)

Candidate Entity Likelihoods:

(**'Q137259', 0.998**), ('Q6999', 0.0), ('Q66311333', 0.0), ('Q488383', 0.0), ...

Top Prediction:

('1241 dysona', 0.965) → (**instance of, 1.000**) → ('Q3863', 0.998) ✓

---

**Question:** what is the place of birth of sam edwards?

**Question Entity:** Q472382 (Sam Edwards, Welsh Physicist)

**Answer Entity** Q23051 (Swansea)

Span Likelihoods:

('edwards', 0.366), (**'sam edwards', 0.332**), ('sam', 0.301), ('what is', 0.0), ('the place', 0.0),  
( 'place', 0.0), ('the place of birth', 0.0), ('place of birth', 0.0), ('birth', 0.0)

Candidate Entity Likelihoods:

('Q3470479', 0.25), ('Q835638', 0.111), ('Q911493', 0.058), ('Q2691159', 0.017),  
( 'Q20812281', 0.016), ('Q1816301', 0.014), ('Q47465190', 0.013), ('Q1118055', 0.011),  
( 'Q58317511', 0.01), (**'Q472382', 0.01**), ('Q27925002', 0.01), ('Q52852726', 0.009), ...

Top Prediction:

('Q3470479', 0.25) → (**place of birth, 1.000**) → ('Q219656', 0.250) ✗

---

Table 2: Example outputs of Rigel-E2E on SimpleQuestions
